# Supplementary material for: CypherBench: Towards Precise Retrieval over Full-scale Modern Knowledge Graphs in the LLM Era
Source: arXiv:2412.18702 source file (2025-04-04)
Supplement: Supplementary file 1 [file appendix-old.tex]

% \section{RETURN Clause Templates}



\section{Schemas of the 11 Property Graphs}

\input{tables/all_graphs}

\input{tables/all_graphs_1}

% \section{Graph Statistics}


\section{Graph Matching Patterns and RETURN Templates}

\input{tables/graph_patterns}

\input{tables/return_patterns}


\section{Detailed CypherBench Statistics}
\input{tables/graph_stats}
\input{tables/question_stats}


\section{Question Rewriting and Verification Prompt}

\section{Error Categories} \label{appendix:error}


\input{tables/error_definition}

\section{Text-to-Cypher Prompt} \label{appendix:prompt}

\section{PSJS Details and Limitations}

\yanlin{Show provenance subgraph examples}
